# Supplementary material for: Fast and Scalable Inference for Spatial Extreme Value Models
Source: arXiv:2110.07051 source file (2024-05-16)
Supplement: Supplementary file 1 [file input-appendix-max-smooth.tex]

In order to use the same implementation of Max-and-Smooth in \cite{jhannesson-etal22}, we adopt their parameterization
\begin{equation}\label{eqn:mult-link}
    (\psi, \tau, \phi) = f(a, b_o, s_o) = (\log(a), \log(b_o/s_o), h(s_o))
\end{equation}
where
\begin{equation}
    h(s_o) = a_{\phi} + b_{\phi}\log[-\log\{1-(s_o+1/2)^{c_{\phi}}\}],
\end{equation}
with $a_{\phi}=0.062376$, $b_{\phi}=0.39563$ and $c_\phi=0.8$.
We refer to \cite{jhannesson-etal22} for how this parameterization is constructed, but note that the $h(\cdot)$ function effectively restricts $\vert s_o < 0.5 \vert$. For the remainder of this section, we refer to Max-and-Smooth as the method in \cite{jhannesson-etal22} implemented with their provided code for both the max and smooth steps. We compare the random effect estimation results of Max-and-Smooth to the results of the proposed Laplace method using the parameterization~\eqref{eqn:mult-link}.

With a different model parameterization, model fitting using the Laplace method is the same as described in Section~\ref{sec:method}, except that the latent Gaussian processes are now imposed on $\psi(\xx)$, $\tau(\xx)$ and $\phi(\xx)$. We apply both Max-and-Smooth and the Laplace method on the same small-scale simulated data in Section~\ref{sec:simulation-medium} with $(a(\xx_i), b(\xx_i), s(\xx_i), \ i=1,\ldots,357)$ transformed via \eqref{eqn:mult-link} into $(\psi(\xx_i), \tau(\xx_i), \phi(\xx_i), \ i=1,\ldots,357)$. 43 out of the 400 locations in Section~\ref{sec:simulation-medium} were removed in this study as their true $s_o$ are greater than $0.5$. All code was run on a personal computer with 3.00GHz Intel Core i7-9700 CPU and 16Gb memory. We drew $1000$ posterior samples for both methods and found Laplace 5 times faster than Max-and-Smooth as implemented in \cite{jhannesson-etal22}.

Figure~\ref{fig:app-eta-estimation} and Table~\ref{tab:comparison-reparam} summarize the estimation results using Max-and-Smooth and Laplace. We find that Laplace outperforms Max-and-Smooth in estimating $\psi(\xx)$ and $\phi(\xx)$ but is worse at estimating $\tau(\xx)$. In terms of the 10-year return level, Laplace under the $(\psi, \tau, \phi)$ parameterization gives a higher mean absolute error (MAE) than Max-and-Smooth for $z_{10}(\xx)$, which is most affected by the estimate of the transformed scale parameter $\tau(\xx)$. That being said, the Laplace method using our original GEV parameterization of $(a, b, s)$ gave an MAE of only $2.18$ for $z_{10}(\xx)$ when fitted to the same dataset (see Section~\ref{sec:simulation-medium}), which is much lower than both Laplace and Max-and-Smooth using the $(\psi, \tau, \phi)$ parameterization. Though Max-and-Smooth has some advantages using the \cite{jhannesson-etal22} parameterization $(\psi, \tau, \phi)$, we note that this parameterization restricts the shape parameter to be small ($<0.5$ in absolute value) and thus might not be suitable for cases where the extreme value observations are more heavy-tailed.
\begin{figure}[htp]
    \centering
    \includegraphics[width=.8\linewidth]{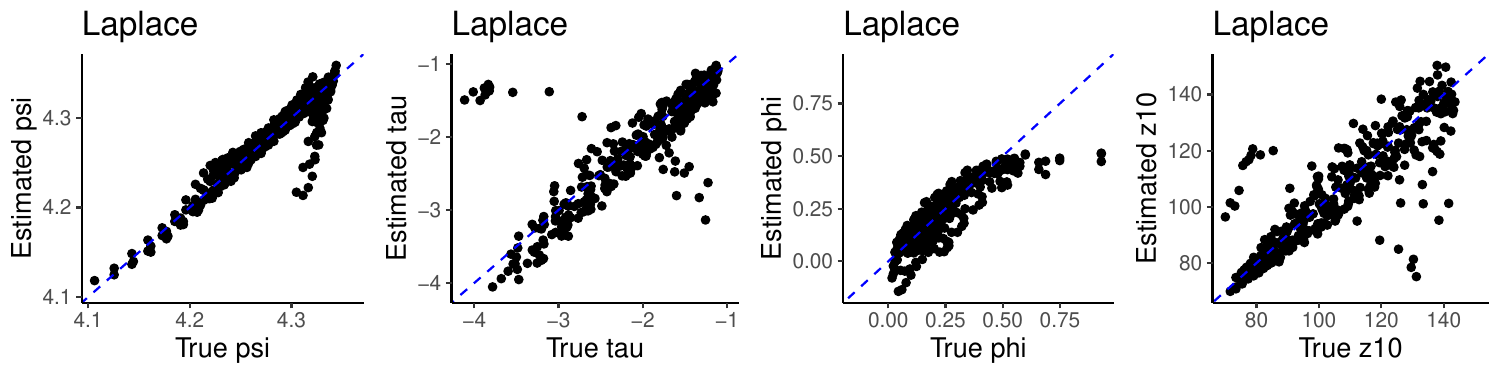}
    \includegraphics[width=.8\linewidth]{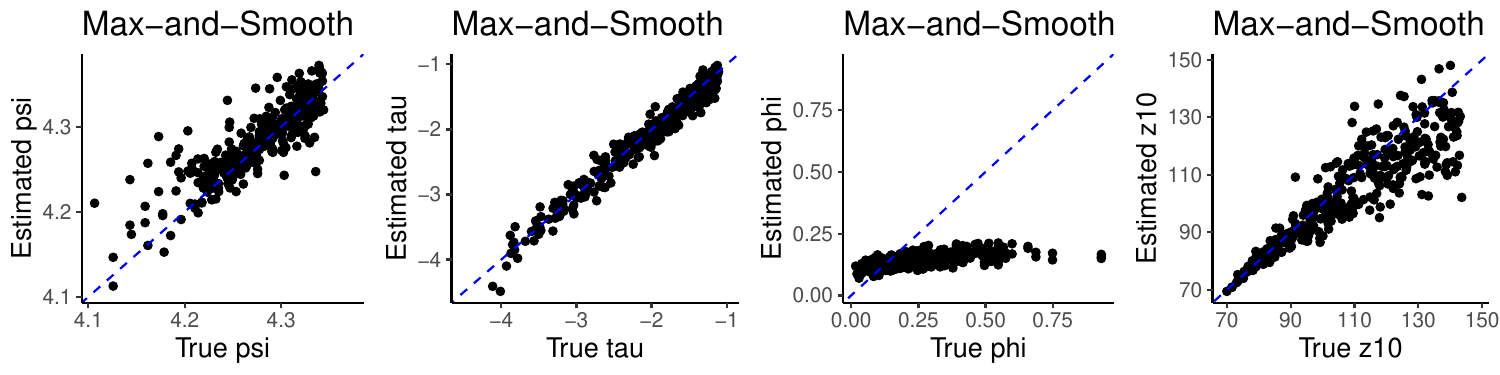}
    \caption{True versus estimated $\psi(\xx_i), \tau(\xx_i), \phi(\xx_i)$ obtained using the Laplace method and the Max-and-Smooth method (implemented with their original code).}
    \label{fig:app-eta-estimation}
\end{figure}

\begin{table}[htp]
\centering
\small
\begin{tabular}{@{}llll@{}} 
\hline
 & Max-and-Smooth & Laplace \\ 
\hline
$\operatorname{MAE}\big(\widehat{\psi}(\xx)\big) = \frac{\sum_{i=1}^n\vert \psi(\xx_i)-\widehat{\psi}(\xx_i)\vert }{n}$& 0.017 & 0.010 \\
$\operatorname{MAE}\big(\widehat{\tau}(\xx)\big) = \frac{\sum_{i=1}^n\vert \tau(\xx_i)-\widehat{\tau}(\xx_i)\vert }{n}$ & 0.11 & 0.26\\
$\operatorname{MAE}\big(\widehat{\phi}(\xx)\big) = \frac{\sum_{i=1}^n\vert \phi(\xx_i)-\widehat{\phi}(\xx_i)\vert }{n}$ & 0.13 & 0.059\\
$\operatorname{MAE}\big(\widehat{z_{10}}(\xx)\big) = \frac{\sum_{i=1}^n\vert z_{10}(\xx_i)-\widehat{z}_{10}(\xx_i)\vert }{n}$ & 6.85 & 7.24\\
\hline
Runtime & 6.85 mins & 1.35 mins\\
\hline
\end{tabular}
\caption{Comparison between Max-and-Smooth and Laplace using the $(\psi, \tau, \phi)$ parameterization introduced in \cite{jhannesson-etal22}.}
\label{tab:comparison-reparam}
\end{table}
